# Supplementary material for: Multi-behavior Graph Contextual Aware Network for Session-based Recommendation
Source: arXiv:2109.11903 source file (2021-09-24)
Supplement: Supplementary file 1 [file appendix.tex]

\begin{appendices}

\section{Search Spaces of the Datasets}\label{appx:dataset}
The \emph{NAS-Bench-101} and \emph{NAS-Bench-201} form their search space differently:
\begin{itemize}
% \begin{inparaitem}
    \item \emph{NAS-Bench-101} donates graph nodes as neural operations, and graph edges as input/output connection, as the left of Fig.\ref{fig:dags} shows. The dataset provides a search space with at most 7 nodes and 9 edges. Except for \emph{input} and \emph{output} nodes, intermediate nodes are one of the operations in \{$1\times 1$ convolution, $3\times 3$ convolution, $3\times 3$ max pooling\}. There are totally 423,624 unique graphs in the search space.
    \item \emph{NAS-Bench-201} uses graph edges to represent both connections and operations, nodes to aggregate intermediate outputs, just like the right of Fig.\ref{fig:dags}. The nodes donate tensor element-wise addition, while edges are operations in \{$1\times 1$ convolution, $3\times 3$ convolution, $3\times 3$ average pooling, skip connection, zeroize\}. This search space consists of 15,625 unique models without considering graph isomorphism. After de-duplicating by graph isomorphism, there are 6,466 unique topology structures.
\end{itemize}

\section{Detailed Baseline Settings}\label{appx:baseline}

Following SOTA of NAS and hyper-parameter optimization methods are used in both \emph{NAS-Bench-101} and \emph{NAS-Bench-201} experiments:

% \begin{inparaitem}
\begin{itemize}
    % \item Global Optimal. The global optimal is selected according to the validation accuracy provided by the datasets.
    \item \textbf{Random Search (RS)} \citep{pmlr-v97-ying19a,Dong2020NAS-Bench-201:}. As reported by many prior works, RS is a competitive algorithm for NAS. We use the implements and settings in \cite{pmlr-v97-ying19a} and \cite{Dong2020NAS-Bench-201:}.
    \item \textbf{Reinforcement Learning (RL)} \citep{zoph2016neural,pmlr-v97-ying19a}. For the RL method, we use the implementation in \citep{pmlr-v97-ying19a}, which directly learns the architecture distribution as action policy, instead of learning an RNN controller as in \citep{zoph2017learning}.
    \item \textbf{Regularized Evolution Algorithm (REA)} \citep{real2019regularized}. The original benchmarks of both datasets show that REA is the state-of-the-art algorithm among the benchmarks  \citep{pmlr-v97-ying19a,Dong2020NAS-Bench-201:}. We inherit the settings from \cite{pmlr-v97-ying19a,Dong2020NAS-Bench-201:}.
    \item \textbf{Bayesian Optimization Hyperband (BOHB)} \citep{falkner2018bohb}. BOHB is a Bayesian optimization method combined with hyperband for fast hyperparameter optimization. We inherit the settings from \cite{pmlr-v97-ying19a,Dong2020NAS-Bench-201:}.
    \item \textbf{Sequential Model-based Algorithm Configuration (SMAC)} \citep{10.1007/978-3-642-25566-3_40}. SMAC is a sequential model-based Bayesian optimization method which employs random forest as the predictor. We inherit the settings from \cite{pmlr-v97-ying19a}.
    \item \textbf{Neural Predictor for Neural Architecture Search (NPNAS)} \citep{wen2019neural}. The NPNAS samples fixed size of architectures from the search space as training data for training a GCN-based surrogate model for once, then freeze the surrogate model and predict the performance of all architectures in the search space to select the best ones. We use the surrogate model we proposed to imitate the method of NPNAS for fair comparison on the searching phrase. We set the training set size to 172 on \emph{NAS-Bench-101} and 128 on \emph{NAS-Bench-201}, which are reported as the optimal values for our search constraint by \citep{wen2019neural}.
\end{itemize}
% \end{inparaitem}

Following baselines are additionally run on \emph{NAS-Bench-101}:

\begin{itemize}
\item \textbf{Neural Architecture Optimization} \citep{NAO}. NAO employs an auto-encoder and perform searching in the learnt embedding space of architectures. We follow the NAS-Bench settings in \cite{luo2020semisupervised}.
\item \textbf{AlphaX} \citep{wang2019alphax}. AlphaX adapts monte-carlo tree search on NAS problem. We keep the settings unchanged from \cite{wang2019alphax}.
\end{itemize}

\section{Experiment Results with Variance}\label{appx:results}

The experiment results on \emph{NAS-Bench-101} and \emph{NAS-Bench-201} with standard deviation is shown in Fig.\ref{fig:search-err}. Note that the variance of the test error on \emph{NAS-Bench-101} is higher than the variance of validation error, since our direct search target is the validation error, and the correlation between validation error and test error is not perfect. Comparing to other baselines, the better mean results of GOAL do not cause higher variance, or even lower, showing the efficiency of GOAL is robust and promising.

\begin{figure}[htbp]
    \centering
    \includegraphics[width=0.49\textwidth]{img/val101.pdf}
    \includegraphics[width=0.49\textwidth]{img/val201.pdf}
    \includegraphics[width=0.49\textwidth]{img/test101.pdf}
    \includegraphics[width=0.49\textwidth]{img/test201.pdf}
    \caption{Comparisons of search efficiency with standard deviation. Left: validation (top) and test (bottom) error of architectures searched on NAS-Bench-101; right: validation (top) and test (bottom) error of architectures searched on NAS-Bench-201.}
    \label{fig:search-err}
\end{figure}

\section{Surrogate Model Performance Accomplished Searching}\label{appx:surrogate}
To analysis the behavior of our surrogate model in the search process, we show the ranking results on all unique architectures in \emph{NAS-Bench-201} of the surrogate model accomplished search process in Fig.\ref{fig:rank_final_1}. For comparison, we also retrained the model with uniformly sampled training data and show the results in Fig.\ref{fig:rank_final_2}. Comparing to the ranking results in Fig.\ref{fig:rank_final_2}, the model accomplished searching performs better on the left-bottom corner, which consists of the best models in the whole search space. Since the architectures with good performance are what we actually concern in the NAS problem, our alternately training strategy in the searching process could enhance the model comparing with the training-once approaches like NPNAS.

\begin{figure}
    \centering
    \begin{subfigure}{0.49\linewidth}
        \includegraphics[width=\linewidth]{img/rankfinal2_.pdf}
        \caption{}\label{fig:rank_final_1}
    \end{subfigure}
    \begin{subfigure}{0.49\linewidth}
        \includegraphics[width=\linewidth]{img/rankfinal2_1.pdf}
        \caption{}\label{fig:rank_final_2}
    \end{subfigure}
    \caption{Left: the ranking result of the model accomplished search process on \emph{NAS-Bench-201}; right: the ranking results of the model retrained with the same size of uniformly sampled training data.}
    \label{fig:rank_final}
\end{figure}

\section{Case Study of the Architecture Transition}\label{appx:case}

Fig.\ref{fig:case} shows the evolution history of an architecture found by GOAL on \emph{NAS-Bench-101}. The case starts at an extremely bad initialization, which directly sends the input to the output. The first step adds several convolution nodes in the company of ResNets-like skip-connections, leading to a meaningful structure. The following steps shrink the architecture to be smaller and fine-tune the connections. As presented in the transition steps, in the \emph{NAS-Bench-101} space, more operations do not always lead to better performance, and the connectivity impacts lot on the final validation accuracy. Notice that only $3\times3$ convolution operations are selected in these architectures, which shows that other operations like max pooling are less helpful for improving accuracy on the tasks in \emph{NAS-Bench-101}.

\begin{figure}[htbp]
    \centering\small
    
    % \import{img/}{cases.pdf_tex}
        \import{img/}{cases.pdf_tex}
    \caption{The 3-step evolution history of a found architecture on \emph{NAS-Bench-101}. 'I', 'O', and 'C3' mean for input node, output node and $3\times3$ convolution node respectively. The green parts are newly added, while dashed parts indicate the deletion.}
    \label{fig:case}
\end{figure}

% \section{Weight-Sharing Strategy \& Results}

% Weight-sharing is a powerful approach for reducing the total time cost on architecture evaluation \citep{pham2018efficient,liu2018darts,dong2019search}. Our GOAL can easily combined with weight-sharing strategy, further improving the overall efficiency of search procedure.

% Our weight sharing strategy generally follows \citet{li2020random,guo2019single} which first trains a super-net model, called training stage, then evaluate architectures as substructures in the super-net, called search stage. The super-net consists of all the possible modules of the architectures in the search space. On training stage, a substructure is uniformly sampled and separated from the super-net in each training iteration for training. The weights are inheritance from the super-net, and only the weights of the selected substructure will be updated. The trained super-net is then be used in the search stage to find the top-performance substructure as the search result.

% Specially, we adapt the algorithm in Alg.\ref{alg:search} to find the best architecture in the search stage. The only difference here is that we do not need to train and evaluate an architecture from scratch; instead we use the substructure separated from the super-net, run a large validation batch, calculate the accuracy as an approximation. The weight sharing version of GOAL runs much faster than many weight sharing approaches like DARTS \citep{liu2018darts} due to the efficient super-net training method, and our search strategy leads better and more robust solution.

\section{Architecture Searched on DARTS Space}\label{appx:darts-res}

\begin{figure}
    \centering
    \begin{subfigure}{0.45\linewidth}
        \includegraphics[width=\linewidth]{img/normal.pdf}
        \caption{}\label{fig:darts-normal}
    \end{subfigure}
    \begin{subfigure}{0.45\linewidth}
        \includegraphics[width=\linewidth]{img/reduction.pdf}
        \caption{}\label{fig:darts-reduce}
    \end{subfigure}
    \caption{Normal (left) and reduction (right) cell found by GOAL on DARTS space.}
    \label{fig:darts-res}
\end{figure}

\end{appendices}
